# Supplementary material for: Adaptive and anisotropic finite element approximation : Theory and algorithms
Source: arXiv:1101.1555 source file (2011-03-04)
Supplement: Supplementary file 3 [file AppendixRectangles.tex]

\section{Appendix : Proof of Lemma \ref{lemmaSeqBlock}}
By $\cQ_n$ we denote  the standard partition of $R_0\in \RR^d$ in $n^d$ identical blocks of diameter $n^{-1} \diam(R_0)$ illustrated on the left in Figure \ref{fig1Rectangles}.
For each $Q \in \cQ_n$ by $x_Q$ we denote the barycenter of $Q$ and we consider the tiling $\cT_Q$ of $\R^d$ formed with the block $n^{-2}R(x_Q)$ and its translates.
We define $\cP_n^1(Q)$ and $\cP_n^1$ as follows
$$
\cP_n^1(Q) := \{R\in \cT_Q \sep R \subset Q\} \ \text{ and } \ \cP_n^1 := \bigcup_{Q\in \cQ_n} \cP_n^1(Q).
$$
Comparing the areas, we obtain
$$
\card (\cP_n^1) = \sum_{Q\in \cQ_n} \cP_n^1(Q) \leq \sum_{Q \in \cQ_n} \frac{|Q|}{|n^{-2} R(x_Q)|} = n^{2 d} \sum_{Q \in \cQ_n} |Q| |R(x_Q)|^{-1}.
$$
From this point, using the continuity of $x \mapsto |R(x)|$, one can easily show that
$
\frac {\# (\cP_n^1)}{n^{2d}} \to \int_{R_0} |R(x)|^{-1} dx
$
as $n \to \infty$. Furthermore, the property \iref{n2Ry} clearly holds. In order to construct $\cP_n^2$, we first define two sets of blocks $\cP_n^{2*}(Q)$ and $\cP_n^{2*}$ as follows
$$
\cP_n^{2*}(Q) := \{R\cap Q \sep R \in \cT_Q \text{ and }R\cap \partial Q\neq \emptyset\} \ \text{ and } \ \cP_n^{2*} := \bigcup_{Q\in \cQ_n} \cP_n^{2*}(Q).
$$
Comparing the surface of $\partial Q$ with the dimensions of $R(x_Q)$, we find that
$$
\#(\cP_n^{2*}(Q)) \leq C n^{d-1}
$$
where $C$ is independent of $n$ and of $Q\in \cQ_n$.
Therefore, $\#(\cP_n^{2*})\leq C n^{2d-1}$. The set of blocks $\cP_n^2$ is then obtained by subdividing each block of $\cP_n^{2*}$ into $o(n^d)$ (for instance, $\lfloor \ln(n)\rfloor^d$) identical sub-blocks, in such a way that $\#(\cP_n^2)$ is $o(n^{2d})$ and that the requirement \iref{smallDiam} is met.

\begin{figure}
    \centering
    \includegraphics[width=4cm,height=4cm]{\pathPic/PaperRectangles/frame.pdf}
    \hspace{1cm}
    \includegraphics[width=4cm,height=4cm]{\pathPic/PaperRectangles/tile.pdf}
    \caption{\label{fig1Rectangles}(Left) the initial uniform (coarse) tiling $\cQ_3$ of $R_0$. (Right) the set of blocks $\cP_n^1$ in green and the set of blocks $\cP_n^{2*}$ in red.}
\end{figure}
